# Supplementary material for: Question Answering as Programming for Solving Time-Sensitive Questions
Source: arXiv:2305.14221 source file (2023-10-20)
Supplement: Supplementary file 1 [file appendix-timeqa-prompt.tex]

% \begingroup
\onecolumn
\begin{table}[tp]
    \centering
    \small
    \begin{supertabular}{p{\linewidth}}
        \toprule
        \underline{\textbf{\textsc{Prompt for Math Word Problems}}} \\
        \vspace{-2mm}
        \vspace{-1mm}Question:Which school did David Jolly go to in Jan 1989?\\ \vspace{-1mm}Question parsing:\\ \vspace{-1mm}```python\\ \vspace{-1mm}query = {"subject": "David Jolly", "relation": "go to school", "object": None, "time": {"start": datetime(1989, 1, 1), "end": datetime(1989, 1, 31)}}\\ \vspace{-1mm}answer\_key = "object"\\ \vspace{-1mm}```\\ \vspace{-1mm}Search:\\ \vspace{-1mm}```python\\ \vspace{-1mm}entities\_to\_search = ["David Jolly"]\\ \vspace{-1mm}```\\ \vspace{-1mm}Generate a background document from Wikipedia to answer the given question:  David Jolly is an American politician who served as the U.S. Representative for Florida's 13th congressional district from 2014 to 2017. He graduated from Indian Rocks Christian School in 1990.\\ \vspace{-1mm}Extract information relevant to the query:\\ \vspace{-1mm}```python\\ \vspace{-1mm}information.append({"subject": "David Jolly", "relation": "go to school", "object": "Indian Rocks Christian School", "time": {"start": datetime(1986, 1, 1), "end": datetime(1990, 12, 31)}})\\ \vspace{-1mm}```\\ \vspace{-1mm}Context: David Jolly David Wilson Jolly ( born October 31 , 1972 ) is an American attorney , former lobbyist , and politician who served as the U.S . Representative for Floridas 13th congressional district , based in Pinellas County , from 2014 to 2017 . He was subsequently reelected in November 2014 , winning 75 percent of the vote , but was unseated in 2016 by former Governor Charlie Crist after court-ordered redistricting made his district more Democratic . In September 2018 , Jolly announced he had left the Republican Party .\\ \vspace{-1mm}Extract information relevant to the query:\\ \vspace{-1mm}There is nothing relevant to the query.\\ \vspace{-1mm}Context: Early life . Jolly was born in Dunedin , Florida , the son of Judith and Lawson Jolly , a Baptist pastor . He received his B.A . degree from Emory University in 1994 and his J.D . degree from the George Mason University School of Law in 2001 .\\ \vspace{-1mm}Extract information relevant to the query:\\ \vspace{-1mm}```python\\ \vspace{-1mm}information.append({"subject": "David Jolly", "relation": "go to school", "object": "Emory University", "time": {"start": datetime(1990, 1, 1), "end": datetime(1994, 12, 31)}})\\ \vspace{-1mm}information.append({"subject": "David Jolly", "relation": "go to school", "object": "George Mason University", "time": {"start": datetime(1995, 1, 1), "end": datetime(2001, 12, 31)}})\\ \vspace{-1mm}```\\ \vspace{-1mm}\\ \vspace{-1mm}Question:Which position did Crispin Blunt hold in Feb 2011?\\ \vspace{-1mm}Question parsing:\\ \vspace{-1mm}```python\\ \vspace{-1mm}query = {"subject": "Crispin Blunt", "relation": "hold position", "object": None, "time": {"start": datetime(2011, 2, 1), "end": datetime(2011, 2, 28)}}\\ \vspace{-1mm}answer\_key = "object"\\ \vspace{-1mm}```\\ \vspace{-1mm}Search:\\ \vspace{-1mm}```python\\ \vspace{-1mm}entities\_to\_search = ["Crispin Blunt"]\\ \vspace{-1mm}```\\ \vspace{-1mm}Generate a background document from Wikipedia to answer the given question: Crispin Blunt is a British Conservative Party politician who has been the Member of Parliament (MP) for Reigate since 1997. In February 2011, he was appointed as the Parliamentary Under-Secretary of State for Prisons and Youth Justice in the Ministry of Justice.\\ \vspace{-1mm}Extract information relevant to the query:\\ \vspace{-1mm}```python\\ \vspace{-1mm}information.append({"subject": "Crispin Blunt", "relation": "hold position", "object": "Member of Parliament", "time": {"start": datetime(1997, 1, 1), "end": None}})\\ \vspace{-1mm}information.append({"subject": "Crispin Blunt", "relation": "hold position", "object": "Parliamentary Under-Secretary of State for Prisons and Youth Justice", "time": {"start": datetime(2011, 2, 1), "end": None}})\\ \vspace{-1mm}```\\ \vspace{-1mm}Context: Crispin Blunt Crispin Jeremy Rupert Blunt ( born 15 July 1960 ) is a British Conservative Party politician . He has served as Member of Parliament ( MP ) for Reigate since 1997 , and from May 2010 to September 2012 he was the Parliamentary Under-Secretary of State for Prisons and Youth Justice within the Ministry of Justice . Blunt first entered the House of Commons at the 1997 general election , when he replaced the then MP Sir George Gardiner who had been deselected by the Constituency Conservative Association Executive Council and joined the Referendum Party .\\ \vspace{-1mm}Extract information relevant to the query:\\ \vspace{-1mm}```python\\ \vspace{-1mm}information.append({"subject": "Crispin Blunt", "relation": "hold position", "object": "Member of Parliament", "time": {"start": datetime(1997, 1, 1), "end": None}})\\ \vspace{-1mm}information.append({"subject": "Crispin Blunt", "relation": "hold position", "object": "Parliamentary Under-Secretary of State for Prisons and Youth Justice", "time": {"start": datetime(2010, 5, 1), "end": datetime(2012, 9, 30)}})\\ \vspace{-1mm}```\\ \vspace{-1mm}\\ \vspace{-1mm}Question:What’s the capital of Klamath County, California between Aug 1854 and Jun 1855?\\ \vspace{-1mm}Question parsing:\\ \vspace{-1mm}```python\\ \vspace{-1mm}query = {"subject": None, "relation": "capital of", "object": "Klamath County, California", "time": {"start": datetime(1854, 8, 1), "end": datetime(1855, 6, 30)}}\\ \vspace{-1mm}answer\_key = "subject"\\ \vspace{-1mm}```\\ \vspace{-1mm}Search:\\ \vspace{-1mm}```python\\ \vspace{-1mm}entities\_to\_search = ["Klamath County"]\\ \vspace{-1mm}```\\ \vspace{-1mm}Failed entities:\\ \vspace{-1mm}```python\\ \vspace{-1mm}failed\_entities = ["Klamath County"]\\ \vspace{-1mm}similar\_entities = ["Klamath County, California", "Klamath County, Oregon", "Klamath Falls, Oregon"]\\ \vspace{-1mm}```\\ \vspace{-1mm}Search:\\ \vspace{-1mm}```python\\ \vspace{-1mm}entities\_to\_search = ["Klamath County, California"]\\ \vspace{-1mm}```\\ \vspace{-1mm}Generate a background document from Wikipedia to answer the given question:  Klamath County, California was a county of California from 1851 to 1874. The county seat was Crescent City from 1851 to 1854 and then Yreka from 1854 to 1874.\\ \vspace{-1mm}Extract information relevant to the query:\\ \vspace{-1mm}```python\\ \vspace{-1mm}information.append({"subject": "Crescent City", "relation": "capital of", "object": "Klamath County, California", "time": {"start": datetime(1851, 1, 1), "end": datetime(1854, 12, 31)}})\\ \vspace{-1mm}information.append({"subject": "Yreka", "relation": "capital of", "object": "Klamath County, California", "time": {"start": datetime(1854, 1, 1), "end": datetime(1874, 12, 31)}})\\ \vspace{-1mm}```\\ \vspace{-1mm}Context: Klamath County , California Klamath County was a county of California from 1851 to 1874 . During its existence , the county seat moved twice and ultimately portions of the territory it once had were carved up and added to nearby counties . The original county seat was Trinidad , on the countys southwestern coast . In 1854 the county seat was moved to Crescent City , because of its larger population . But the western portion of the county was unrepresentative of the mining interests in the eastern portion of the county , and so , in 1856 , the county seat was moved inland , to Orleans Bar , now Orleans . In 1857 , Del Norte County , including Crescent City , was split off from Klamath County . In 1874 Klamath County was finally abolished , divided between Siskiyou and Humboldt counties .\\ \vspace{-1mm}Extract information relevant to the query:\\ \vspace{-1mm}```python\\ \vspace{-1mm}information.append({"subject": "Trinidad", "relation": "capital of", "object": "Klamath County, California", "time": {"start": datetime(1851, 1, 1), "end": datetime(1853, 12, 31)}})\\ \vspace{-1mm}information.append({"subject": "Crescent City", "relation": "capital of", "object": "Klamath County, California", "time": {"start": datetime(1854, 1, 1), "end": datetime(1855, 12, 31)}})\\ \vspace{-1mm}information.append({"subject": "Orleans", "relation": "capital of", "object": "Klamath County, California", "time": {"start": datetime(1856, 1, 1), "end": datetime(1856, 12, 31)}})\\ \vspace{-1mm}```

        \\
        \bottomrule
    \end{supertabular}
        \caption{
    Few-shot exemplars for full chain of thought prompt for math word problems. This set of exemplars was used for all math word problem datasets except AQuA. 
    }
    \label{tab:appendix-timeqa-prompt}
\end{table}
% \endgroup

\begin{longtable}{p\linewidth} 
\hline
\small
        \vspace{-1mm}Question:Which school did David Jolly go to in Jan 1989?\\ \vspace{-1mm}Question parsing:\\ \vspace{-1mm}```python\\ \vspace{-1mm}query = {"subject": "David Jolly", "relation": "go to school", "object": None, "time": {"start": datetime(1989, 1, 1), "end": datetime(1989, 1, 31)}}\\ \vspace{-1mm}answer\_key = "object"\\ \vspace{-1mm}```\\ \vspace{-1mm}Search:\\ \vspace{-1mm}```python\\ \vspace{-1mm}entities\_to\_search = ["David Jolly"]\\ \vspace{-1mm}```\\ \vspace{-1mm}Generate a background document from Wikipedia to answer the given question:  David Jolly is an American politician who served as the U.S. Representative for Florida's 13th congressional district from 2014 to 2017. He graduated from Indian Rocks Christian School in 1990.\\ \vspace{-1mm}Extract information relevant to the query:\\ \vspace{-1mm}```python\\ \vspace{-1mm}information.append({"subject": "David Jolly", "relation": "go to school", "object": "Indian Rocks Christian School", "time": {"start": datetime(1986, 1, 1), "end": datetime(1990, 12, 31)}})\\ \vspace{-1mm}```\\ \vspace{-1mm}Context: David Jolly David Wilson Jolly ( born October 31 , 1972 ) is an American attorney , former lobbyist , and politician who served as the U.S . Representative for Floridas 13th congressional district , based in Pinellas County , from 2014 to 2017 . He was subsequently reelected in November 2014 , winning 75 percent of the vote , but was unseated in 2016 by former Governor Charlie Crist after court-ordered redistricting made his district more Democratic . In September 2018 , Jolly announced he had left the Republican Party .\\ \vspace{-1mm}Extract information relevant to the query:\\ \vspace{-1mm}There is nothing relevant to the query.\\ \vspace{-1mm}Context: Early life . Jolly was born in Dunedin , Florida , the son of Judith and Lawson Jolly , a Baptist pastor . He received his B.A . degree from Emory University in 1994 and his J.D . degree from the George Mason University School of Law in 2001 .\\ \vspace{-1mm}Extract information relevant to the query:\\ \vspace{-1mm}```python\\ \vspace{-1mm}information.append({"subject": "David Jolly", "relation": "go to school", "object": "Emory University", "time": {"start": datetime(1990, 1, 1), "end": datetime(1994, 12, 31)}})\\ \vspace{-1mm}information.append({"subject": "David Jolly", "relation": "go to school", "object": "George Mason University", "time": {"start": datetime(1995, 1, 1), "end": datetime(2001, 12, 31)}})\\ \vspace{-1mm}```\\ \vspace{-1mm}\\ \vspace{-1mm}Question:Which position did Crispin Blunt hold in Feb 2011?\\ \vspace{-1mm}Question parsing:\\ \vspace{-1mm}```python\\ \vspace{-1mm}query = {"subject": "Crispin Blunt", "relation": "hold position", "object": None, "time": {"start": datetime(2011, 2, 1), "end": datetime(2011, 2, 28)}}\\ \vspace{-1mm}answer\_key = "object"\\ \vspace{-1mm}```\\ \vspace{-1mm}Search:\\ \vspace{-1mm}```python\\ \vspace{-1mm}entities\_to\_search = ["Crispin Blunt"]\\ \vspace{-1mm}```\\ \vspace{-1mm}Generate a background document from Wikipedia to answer the given question: Crispin Blunt is a British Conservative Party politician who has been the Member of Parliament (MP) for Reigate since 1997. In February 2011, he was appointed as the Parliamentary Under-Secretary of State for Prisons and Youth Justice in the Ministry of Justice.\\ \vspace{-1mm}Extract information relevant to the query:\\ \vspace{-1mm}```python\\ \vspace{-1mm}information.append({"subject": "Crispin Blunt", "relation": "hold position", "object": "Member of Parliament", "time": {"start": datetime(1997, 1, 1), "end": None}})\\ \vspace{-1mm}information.append({"subject": "Crispin Blunt", "relation": "hold position", "object": "Parliamentary Under-Secretary of State for Prisons and Youth Justice", "time": {"start": datetime(2011, 2, 1), "end": None}})\\ \vspace{-1mm}```\\ \vspace{-1mm}Context: Crispin Blunt Crispin Jeremy Rupert Blunt ( born 15 July 1960 ) is a British Conservative Party politician . He has served as Member of Parliament ( MP ) for Reigate since 1997 , and from May 2010 to September 2012 he was the Parliamentary Under-Secretary of State for Prisons and Youth Justice within the Ministry of Justice . Blunt first entered the House of Commons at the 1997 general election , when he replaced the then MP Sir George Gardiner who had been deselected by the Constituency Conservative Association Executive Council and joined the Referendum Party .\\ \vspace{-1mm}Extract information relevant to the query:\\ \vspace{-1mm}```python\\ \vspace{-1mm}information.append({"subject": "Crispin Blunt", "relation": "hold position", "object": "Member of Parliament", "time": {"start": datetime(1997, 1, 1), "end": None}})\\ \vspace{-1mm}information.append({"subject": "Crispin Blunt", "relation": "hold position", "object": "Parliamentary Under-Secretary of State for Prisons and Youth Justice", "time": {"start": datetime(2010, 5, 1), "end": datetime(2012, 9, 30)}})\\ \vspace{-1mm}```\\ \vspace{-1mm}\\ \vspace{-1mm}Question:What’s the capital of Klamath County, California between Aug 1854 and Jun 1855?\\ \vspace{-1mm}Question parsing:\\ \vspace{-1mm}```python\\ \vspace{-1mm}query = {"subject": None, "relation": "capital of", "object": "Klamath County, California", "time": {"start": datetime(1854, 8, 1), "end": datetime(1855, 6, 30)}}\\ \vspace{-1mm}answer\_key = "subject"\\ \vspace{-1mm}```\\ \vspace{-1mm}Search:\\ \vspace{-1mm}```python\\ \vspace{-1mm}entities\_to\_search = ["Klamath County"]\\ \vspace{-1mm}```\\ \vspace{-1mm}Failed entities:\\ \vspace{-1mm}```python\\ \vspace{-1mm}failed\_entities = ["Klamath County"]\\ \vspace{-1mm}similar\_entities = ["Klamath County, California", "Klamath County, Oregon", "Klamath Falls, Oregon"]\\ \vspace{-1mm}```\\ \vspace{-1mm}Search:\\ \vspace{-1mm}```python\\ \vspace{-1mm}entities\_to\_search = ["Klamath County, California"]\\ \vspace{-1mm}```\\ \vspace{-1mm}Generate a background document from Wikipedia to answer the given question:  Klamath County, California was a county of California from 1851 to 1874. The county seat was Crescent City from 1851 to 1854 and then Yreka from 1854 to 1874.\\ \vspace{-1mm}Extract information relevant to the query:\\ \vspace{-1mm}```python\\ \vspace{-1mm}information.append({"subject": "Crescent City", "relation": "capital of", "object": "Klamath County, California", "time": {"start": datetime(1851, 1, 1), "end": datetime(1854, 12, 31)}})\\ \vspace{-1mm}information.append({"subject": "Yreka", "relation": "capital of", "object": "Klamath County, California", "time": {"start": datetime(1854, 1, 1), "end": datetime(1874, 12, 31)}})\\ \vspace{-1mm}```\\ \vspace{-1mm}Context: Klamath County , California Klamath County was a county of California from 1851 to 1874 . During its existence , the county seat moved twice and ultimately portions of the territory it once had were carved up and added to nearby counties . The original county seat was Trinidad , on the countys southwestern coast . In 1854 the county seat was moved to Crescent City , because of its larger population . But the western portion of the county was unrepresentative of the mining interests in the eastern portion of the county , and so , in 1856 , the county seat was moved inland , to Orleans Bar , now Orleans . In 1857 , Del Norte County , including Crescent City , was split off from Klamath County . In 1874 Klamath County was finally abolished , divided between Siskiyou and Humboldt counties .\\ \vspace{-1mm}Extract information relevant to the query:\\ \vspace{-1mm}```python\\ \vspace{-1mm}information.append({"subject": "Trinidad", "relation": "capital of", "object": "Klamath County, California", "time": {"start": datetime(1851, 1, 1), "end": datetime(1853, 12, 31)}})\\ \vspace{-1mm}information.append({"subject": "Crescent City", "relation": "capital of", "object": "Klamath County, California", "time": {"start": datetime(1854, 1, 1), "end": datetime(1855, 12, 31)}})\\ \vspace{-1mm}information.append({"subject": "Orleans", "relation": "capital of", "object": "Klamath County, California", "time": {"start": datetime(1856, 1, 1), "end": datetime(1856, 12, 31)}})        \\ \vspace{-1mm}```
        \\
\caption{Your caption here} % needs to go inside longtable environment
\label{tab:myfirstlongtable}
\end{longtable}
